# Supplementary material for: Differentially Private Maximal Information Coefficients
Source: arXiv:2206.10685 source file (2022-06-21)
Supplement: Supplementary file 1 [file appendix-functions.tex]

% functions for synthetic data

\subsubsection{Synthetic Data Functional Relationships}

List of functional relationships:
\begin{itemize}
\item
  F1: $f(x) = 0.2 \cdot \sin(12x - 6) + 1.1(x-1) + 1$
\item
  F2: $f(x) = 0.15 \cdot \sin(11x \cdot \pi) + (x + 0.05)$
\item
  F3: $f(x) = 0.1 \cdot \sin(48x) + 2(x - 0.05)$
\item
  F4: $f(x) = 0.2 \cdot \sin(48x) + 2(x - 0.05)$
\item
  F5: $f(x) = 0.4 \cdot \cos(7x \cdot \pi) + 0.5$
\item
  F6: $f(x) = 0.4 \cdot \cos(14x \cdot \pi) + 0.5$
\item
  F7: $f(x) = 10 \cdot {(x - 0.6)}^3 + 2 \cdot {x}^2 + (1.5 - 3x)$
\item
  F8: $f(x) = 4 \cdot (10 \cdot {(x - 0.6)}^3 + 2 \cdot {x}^2 + (1.5 - 3x)) - 1.4 $
\item
  F9: $if x \leq 0.99 then f(x) = \frac{x}{99}, else f(x) = 99x - 98$
\item
  F10: $f(x) = {2}^x - 1$
\item
  F11: $f(x) = {8}^(x - 0.3) - 1$
\item
  F12: $f(x) = x$
\item
  F13: $f(x) = 4 \cdot {(x - 0.5)}^2 + 0.1$
\item
  F14: $f(x) = 0.4 \cdot \sin(9x \cdot \pi) + 0.5$
\item
  F15: $f(x) = 0.4 \cdot \sin(8x \cdot \pi) + 0.5$
\item
  F16: $f(x) = 0.4 \cdot \sin(16x \cdot \pi) + 0.5$
\item
  F17: $if x < 0.491 then f(x) = 0.05, else if x > 0.509 then f(x) = 0.95, else f(x) = 50 \cdot (x - 0.5) + 0.5$
\item
  F18: $f(x) = 0.4 \cdot \cos(5x \cdot \pi \cdot (1 + x)) + 0.5$
\item
  F19: $f(x) = 0.4 \cdot \sin(6x \cdot \pi \cdot (1 + x)) + 0.5$
\item
  F20: $if x \leq 0.0528 then f(x) = 18x, else if x \geq 0.1 then f(x) = -1 \cdot \frac{x}{9} + \frac{1}{9}, else f(x) = -18x + 1.9$
\item
  F21: $if x \leq 0.0051 then f(x) = 190x, else if x \geq 0.01 then f(x) = -1 \cdot \frac{x}{99} + \frac{1}{99}, else f(x) = -198x + 1.99$

\end{itemize}

%%% Local Variables:
%%% mode: latex
%%% TeX-master: "../dpmic-main"
%%% End:
